# Supplementary material for: Impact of Surface Adsorbates and Dimensionality on Templating of Halide Perovskites
Source: arXiv:2405.08336 ancillary file (2024-05-14)
Supplement: Supplementary file 1 [file supporting-information.pdf]

# Supplemental Material:

# Impact of Surface Adsorbates and Dimensionality in Templating of Halide Perovskites

Erik Fransson[1], Julia Wiktor[1], and Paul Erhart[1]

[1] *Department of Physics, Chalmers University of Technology, SE-41296, Gothenburg, Sweden*

May 9, 2024

# Contents

**1 NEP model** **2**

**2 Additional analysis of cooling simulations** **3**

**3 Transitions in additional systems** **7**

**Supplemental References** **11**

# 1 NEP model

We construct a neuroevolution potential (NEP) model using the bootstrapping and active learning strategy outlined in Ref. 1 using the GPUMD software.[2–4] The resulting training and validation errors obtained by cross validation with 10 folds are shown in Fig. S1.

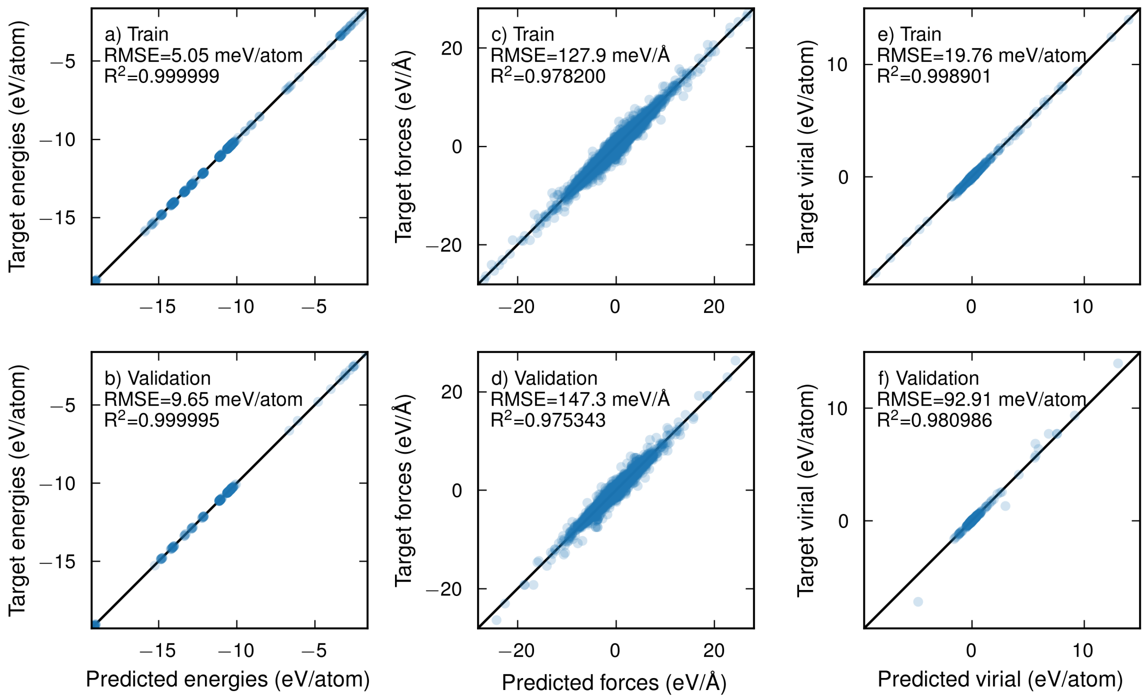


Figure S1: Parity plots for total energies, forces and virials for training and validation sets.

## 2 Additional analysis of cooling simulations

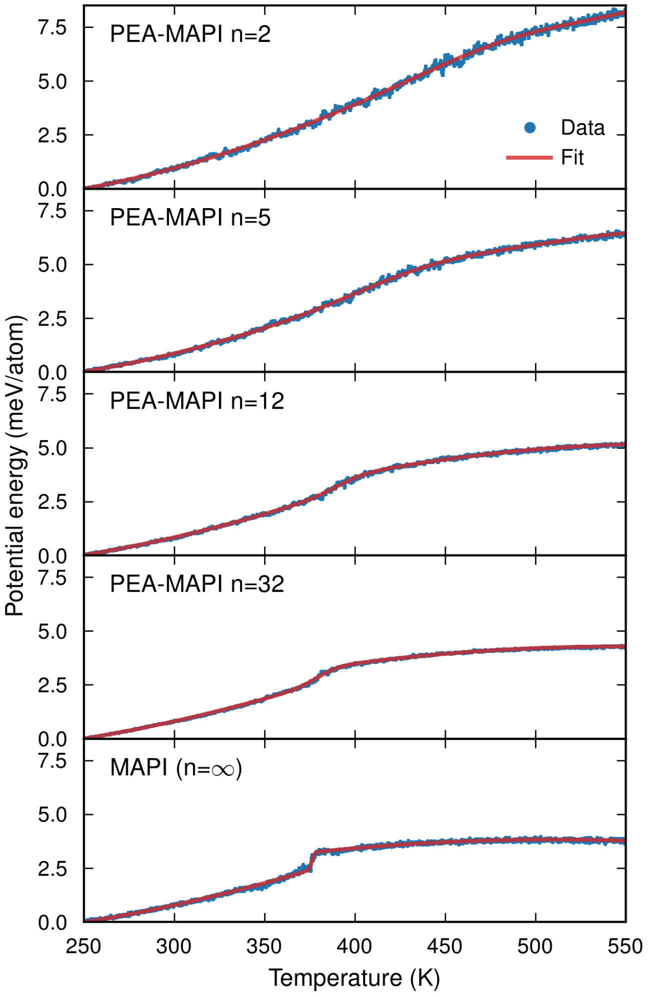


Figure S2: Potential energy data from cooling simulations averaged using a gliding window with a size corresponding to 0.4 K and fits to two polynomials splined together with an error function.

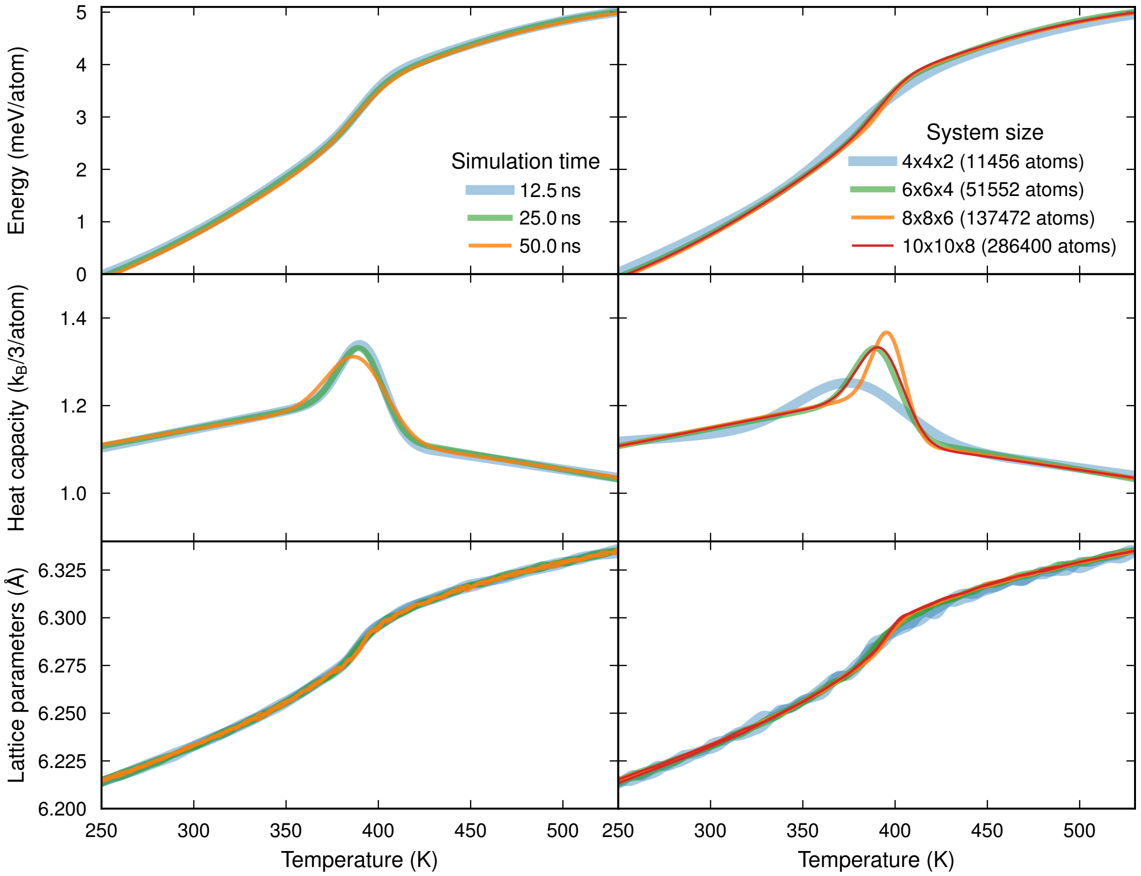


Figure S3: Convergence of potential energy, heat capacity and in-plane lattice-parameters with respect to simulation time (left) and system size (right) for PEA-MAPbI$_3$ $n = 12$. Unless specified the system size and simulation length are the same as used in the remainder of this paper, i.e., $6 \times 6 \times 4$ and 25 ns.

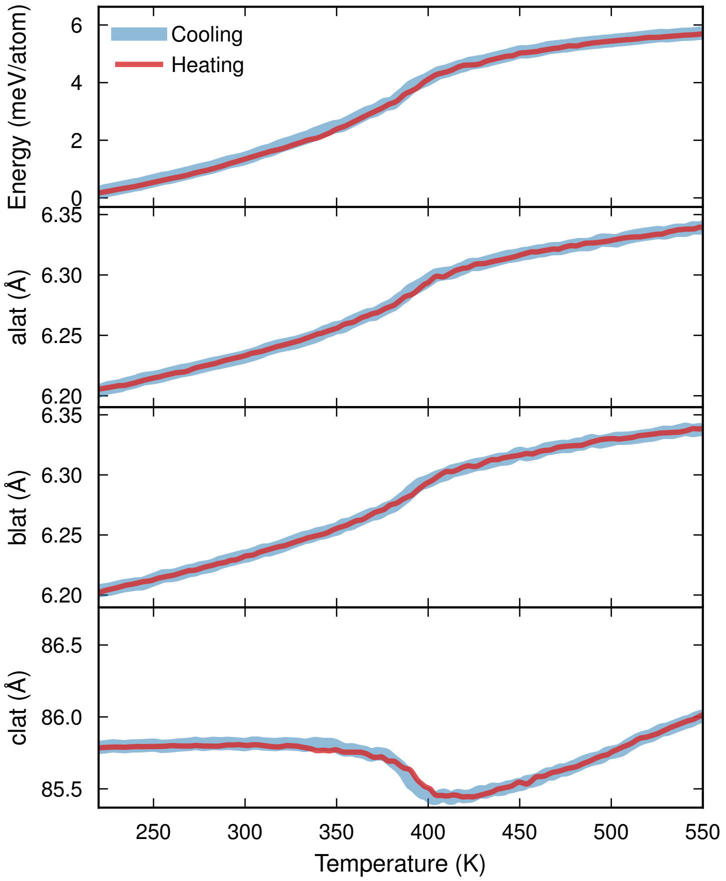


Figure S4: Thermodynamic properties from heating and cooling runs for PEA-MAP$bI_3$ with $n = 12$.

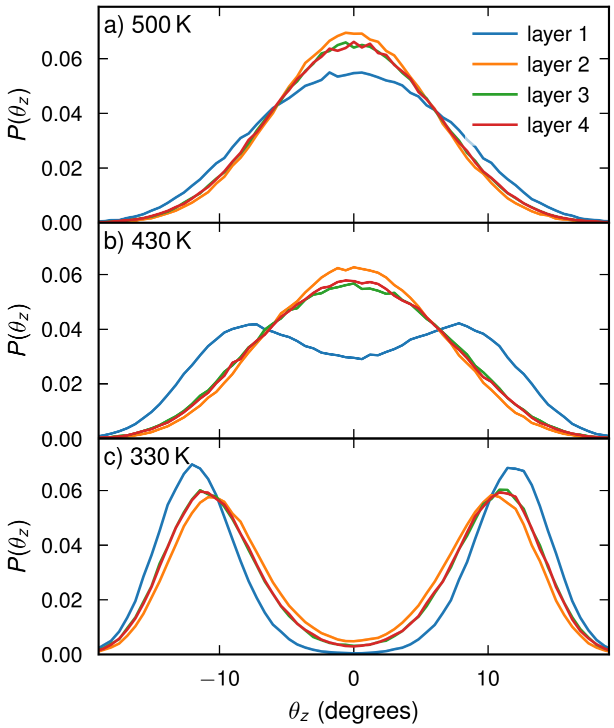


Figure S5: Probability distribution over the octahedral tilt angles, $P(\theta_z)$, for each symmetrically distinct layer in PEA-MAPbI$_3$ with $n = 8$ at (a) 500 K, (b) 430 K and (c) 330 K. Here, layer 1 refers to the perovskite layer closes to the organic linker molecule.

# 3 Transitions in additional systems

Here, we consider the cooling runs of phenylmethylammonium $C_6H_5(CH_2)NH_3$ (PMA)-$MAPbI_3$, butylammonium $CH_3(CH_2)_3NH_3$ (BA)-$MAPbI_3$ and the $MAPI_3$ surface {001} surface. We note that there is some uncertainty of about $\pm 10$ K when determining the transition temperatures from the tilt angle analysis as done here due to the stochastic nature of the molecular dynamics (MD) simulations. For example, perovskite regions separated by the linker can undergo the transitions at slightly different points of time in the MD simulations, and the presence of anti-phase boundaries leads to small changes in the transition temperature.

One should also note that the NEP model overestimates the $MAPbI_3$ bulk transition temperature by about 40 K compared to experiment. We therefore emphasize that these results should be interpreted in a qualitative or semi-qualitative manner.

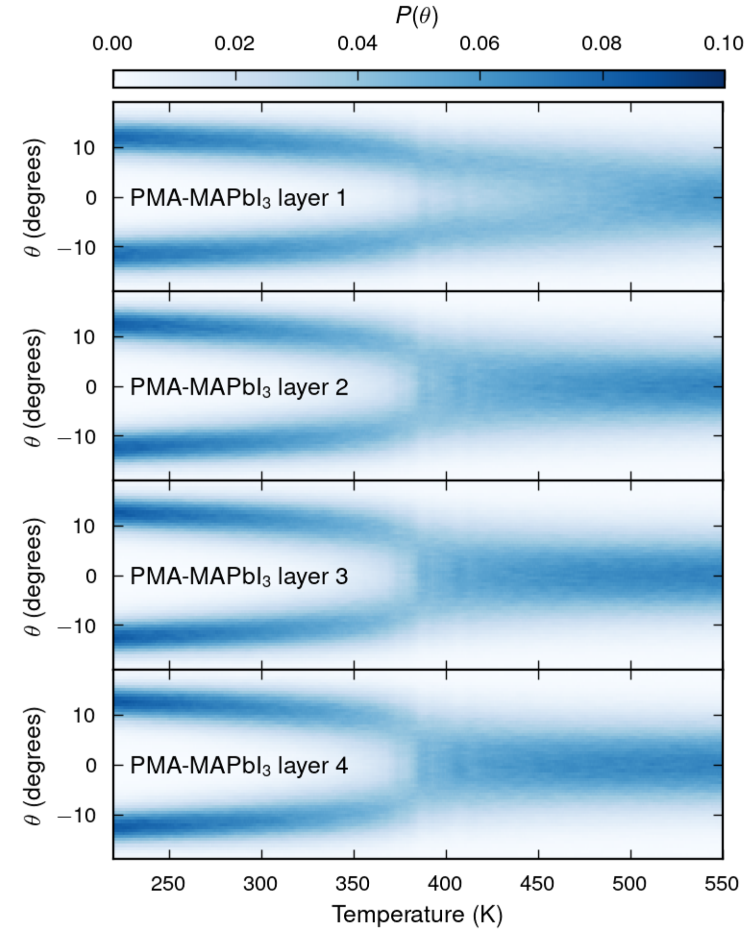


Figure S6: Probability distribution over the octahedral tilt angles, $P(\theta)$, as a function of temperature for PMA-$MAPbI_3$ with $n = 8$.

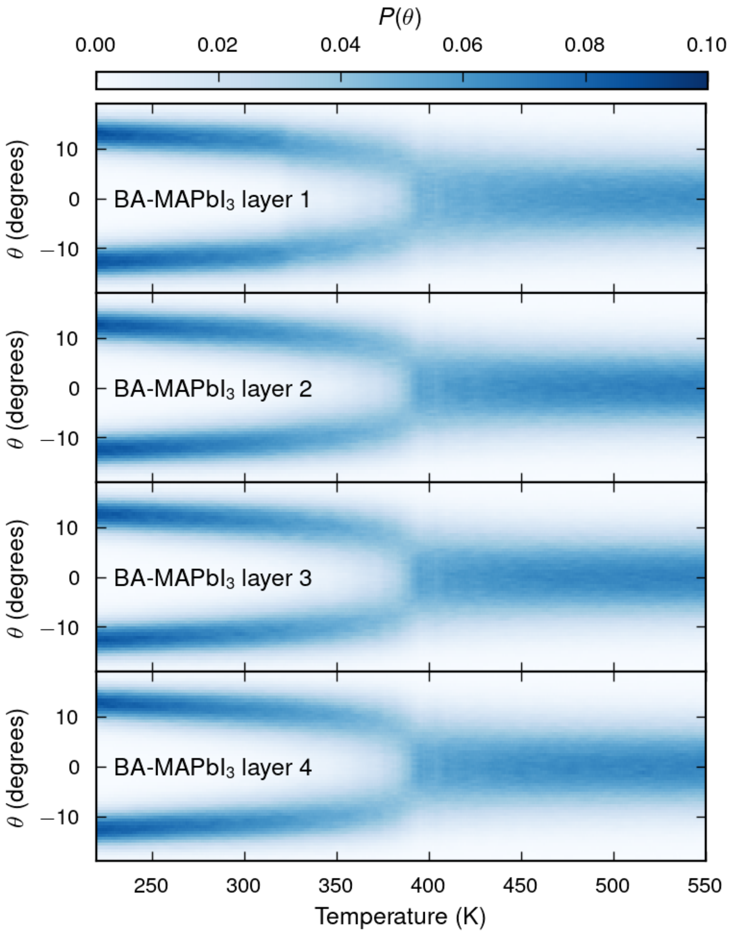


Figure S7: Probability distribution over the octahedra tilt angles, $P(\theta)$, as a function of temperature for BA-$MAPbI_3$ with $n = 8$.

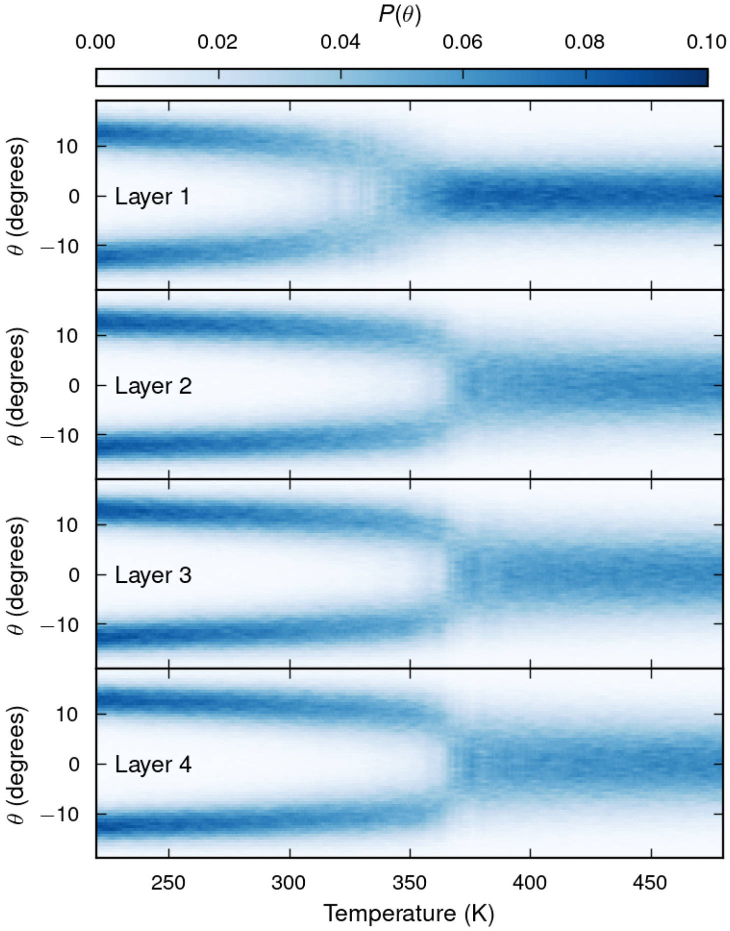


Figure S8: Probability distribution over the octahedral tilt angles, $P(\theta)$, as a function of temperature for a pure $MAPbI_3$ {001} surface with $MAI_2$ termination with a total of 16 perovskite unit cells in the $z$-direction. Here, the tilt angles are shown for the first four layers starting with the top-most surface layer.

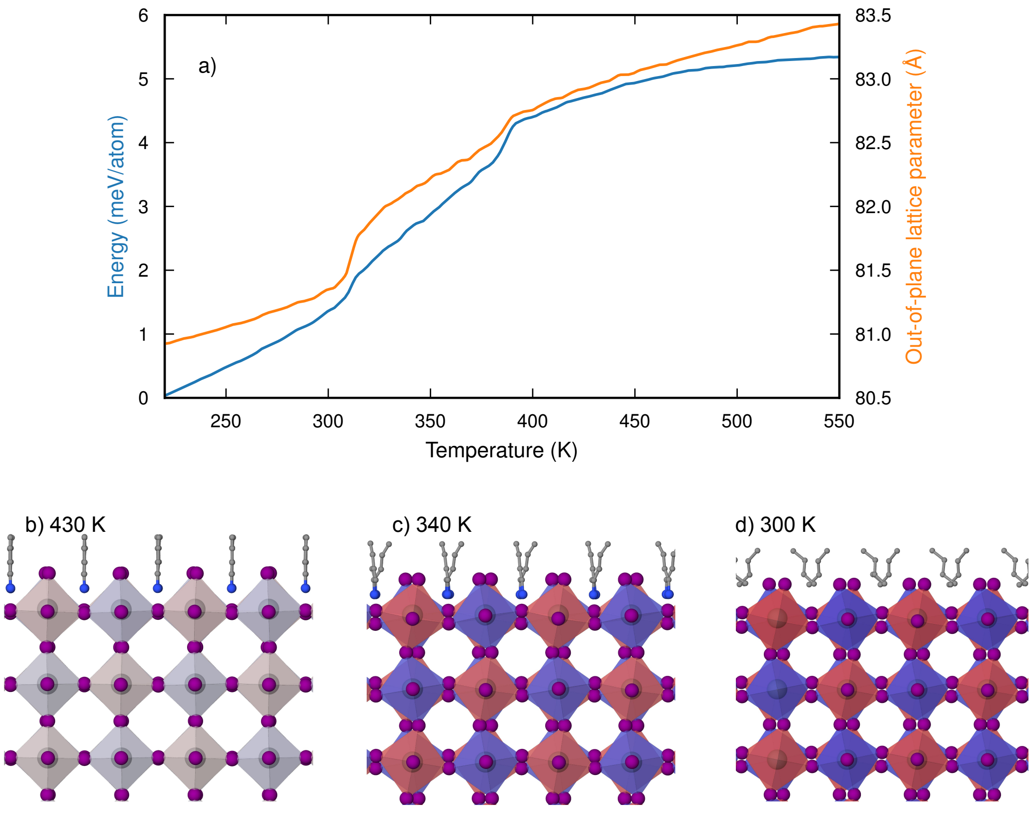


Figure S9: (a) Energy and out-of-plane lattice parameter for BA-MAP$bI_3$ with $n = 12$. At about 380 K one observes the transition between the untilted and the tilted structure, and around 300 K there is a transition related to freezing in the BA molecules in a "bent" configuration leading to a significant drop in the out-of-plane lattice parameter. (b–d) Average atomic configurations at (b) 430 K, (c) 340 K and (d) 300 K. Red and blue octahedra indicate negative and positive tilt angles (ranging from $-20$ to $20°$), respectively, whereas gray implies tilt angles close to zero.

# Supplemental References

[1] Erik Fransson, Julia Wiktor, and Paul Erhart. Phase transitions in inorganic halide perovskites from machine-learned potentials. *The Journal of Physical Chemistry C*, 127(28):13773–13781, July 2023. doi: 10.1021/acs.jpcc.3c01542.

[2] Zheyong Fan, Zezhu Zeng, Cunzhi Zhang, Yanzhou Wang, Keke Song, Haikuan Dong, Yue Chen, and Tapio Ala-Nissila. Neuroevolution machine learning potentials: Combining high accuracy and low cost in atomistic simulations and application to heat transport. *Physical Review B*, 104:104309, Sep 2021. doi: 10.1103/PhysRevB.104.104309.

[3] Zheyong Fan. Improving the accuracy of the neuroevolution machine learning potential for multi-component systems. *Journal of Physics: Condensed Matter*, 34(12):125902, jan 2022. doi: 10.1088/1361-648x/ac462b.

[4] Zheyong Fan, Yanzhou Wang, Penghua Ying, Keke Song, Junjie Wang, Yong Wang, Zezhu Zeng, Ke Xu, Eric Lindgren, J. Magnus Rahm, Alexander J. Gabourie, Jiahui Liu, Haikuan Dong, Jianyang Wu, Yue Chen, Zheng Zhong, Jian Sun, Paul Erhart, Yanjing Su, and Tapio Ala-Nissila. GPUMD: A package for constructing accurate machine-learned potentials and performing highly efficient atomistic simulations. *The Journal of Chemical Physics*, 157(11):114801, September 2022. doi: 10.1063/5.0106617.
